# Supplementary material for: Online Nonparametric Regression with General Loss Functions
Source: arXiv:1501.06598 source file (2015-01-26)
Supplement: Supplementary file 1 [file appendix_algos.tex]

\begin{proof}[\textbf{Proof of Proposition \ref{prop:recipe}}]
Notice that the above recipe closely follows the notion of relaxation provided in \citep{rakhlin2012relax}. All we need to do is check that the relaxation derived satisfies admissibility and initial conditions. By Step 1 of the recipe, since the offset Rademacher relaxation is admissible to start with, the derived relaxation also satisfies initial condition. To show admissibility condition notice that the set $[-B,B]$ is compact and convex and $(\hat{y}_t - y_t)^2 + \Rel{n}{x_{1:t},y_{1:t}}$ is a convex function of $\hat{y}_t$. Hence applying minimax theorem, we see that,
\begin{align*}
&\inf_{\hat{y}_t \in [-B,B]}  \sup_{y_t \in [-B,B]}\left\{ (\hat{y}_t - y_t)^2 + \Rel{n}{x_{1:t},y_{1:t}} \right\} \\
& = \sup_{p_t \in \Delta([-B,B])} \inf_{\hat{y}_t}\left\{ \Es{y_t \sim p_t}{(\hat{y}_t - y_t)^2 + \Rel{n}{x_{1:t},y_{1:t}}} \right\}\\
&  = \sup_{p_t \in \Delta([-B,B])}\left\{ \inf_{\hat{y}_t}\ \Es{y_t \sim p_t}{(\hat{y}_t - y_t)^2} + \Es{y_t \sim p_t}{\Rel{n}{x_{1:t},y_{1:t}}} \right\}\\
&  = \sup_{p_t \in \Delta([-B,B])}\left\{  \Es{y_t \sim p_t}{\left(\Es{y_t \sim p_t}{y_t} - y_t\right)^2} + \Es{y_t \sim p_t}{\Rel{n}{x_{1:t},y_{1:t}}} \right\}
\end{align*}
Hence the admissibility condition can be rewritten as :
\begin{align*}
\forall x_t \in \X,~~~~ \sup_{p_t \in \Delta([-B,B])}\left\{  \Es{y_t \sim p_t}{\left(\Es{y_t \sim p_t}{y_t} - y_t\right)^2} + \Es{y_t \sim p_t}{\Rel{n}{x_{1:t},y_{1:t}}} \right\} \le \Rel{n}{x_{1:t-1},y_{1:t-1}}. 
\end{align*}
\end{proof}
